# Supplementary material for: Machine-learned tuning to protected states by probing noise resilience
Source: arXiv:2511.01531 source file (2025-11-03)
Supplement: Supplementary file 1 [file supplementary.pdf]

# Supplemental Material for "Machine-learned tuning to protected states by probing noise resilience"


Rodrigo A. Dourado,[1,*] Nicolàs Martínez-Valero,[2] Jacob Benestad,[3]
Martin Leijnse,[4] Jeroen Danon,[3] and Rubén Seoane Souto[2]

[1] *Departamento de Física, Universidade Federal de Minas Gerais, C. P. 702, 30123-970, Belo Horizonte, MG, Brazil*
[2] *Instituto de Ciencia de Materiales de Madrid (ICMM), Consejo Superior de Investigaciones Científicas (CSIC), Sor Juana Inés de la Cruz 3, 28049 Madrid, Spain*
[3] *Department of Physics, Norwegian University of Science and Technology, Trondheim NO-7491, Norway*
[4] *Division of Solid State Physics and NanoLund, Lund University, S-22100 Lund, Sweden*



(Dated: November 2, 2025)


## A. THE CMA-ES ALGORITHM

The covariance matrix adaptation evolutionary strategy (CMA-ES) is a gradient-free optimization algorithm with qualities that make it well-suited for automatic tuning of multiple gate voltages in quantum experiments [1–4]. Firstly, being a stochastic method and not relying on gradients makes it more robust to non-convex loss functions that are likely to arise when dealing with realistic devices and possible measurement noise. Secondly, the CMA-ES algorithm is both conceptually simple and easy to use, with available software implementations allowing for a "plug-and-play" application of the method (where it often suffices to use mostly default settings to obtain satisfactory results). Thirdly, CMA-ES requires little device-specific information about the loss landscape, allowing us to be largely agnostic about the optimization problem details.

In broad terms, the CMA-ES algorithm works as follows (see Fig. S1): (i) At each generation $g$ a population of candidate solutions (here voltage configurations $\{\varepsilon_1, \varepsilon_2, \dots\}$) is sampled from a multivariate normal (MvN) distribution parameterized by the mean $\mu(g)$ and covariance matrix $\Sigma(g) = \sigma(g)C(g)$, where the covariance matrix is decomposed as a product of a "step size" $\sigma(g)$ and a rescaled covariance matrix $C(g)$. (ii) A measurement of each candidate solution is performed (in simulation or experiment), and the loss function is evaluated with respect to the measurement outcome. (iii) After evaluating each candidate, their resulting loss function values are compared and ranked. (iv) Based on the location of the best-ranked solutions, the MvN is updated by changing $\mu(g)$, $\sigma(g)$, and $C(g)$ to move the "search area" more towards these solutions, increase/decrease its size as necessary and adjust its shape to direct the search more towards the best solutions. The four points are then repeated for the next generation, $g + 1$, and so on, until the search converges to a minimum of the loss function.

We work with the `CMAEvolutionStrategy` function from the `cma.evolution_strategy` Python package, using the following configurations. The initial step-size $\sigma$ is set to $\Delta$, the population $n_{\mathrm{pop}}$ to 20, and we work with a maximum of $5,000$ generations. Additionally, we use the settings `'CMA_diagonal: 10'` to speed the initial search of the algorithm by avoiding correlations in the $C$ matrix, `'CMA_rankmu: 0.05'` and `'CMA_rankone: 0.1'` to smoothen the adaptation on the step size $\sigma$, and `'tolconditioncov: 1e6'` to avoid one of the axes assuming large values in comparison to the other (such as some QD levels being severely detuned, for instance). Finally, we add `'tolx: 1e-3'` as a condition to stop the search. For the 3-site chain, this value is changed to `'1.2e-3'`for $\beta = 1$ and to `'2e-3'` for $\beta = 2$. Finally, for the chains with $N \geq 5$, we assume symmetric QD levels from left to right to reduce the number of variables to optimize.

## B. QUANTITATIVE SUMMARY OF RESULTS

Below, we provide tables that summarize the results for each MBS quantity, in terms of the median value and standard deviations of the final generation, for each figure of the text.


* dourado.rodrigo.a@gmail.com

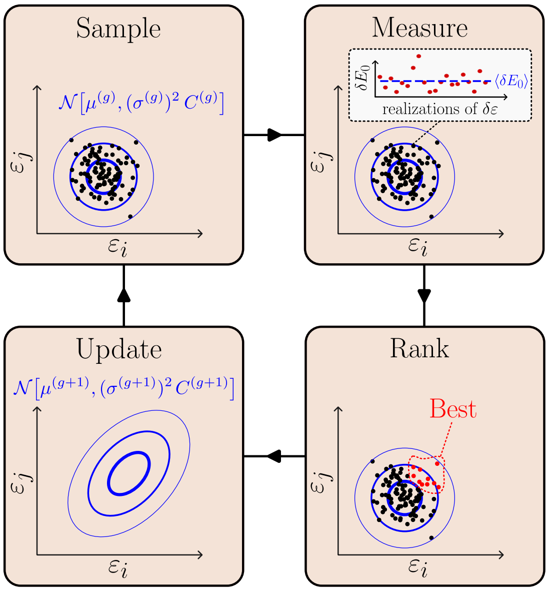


FIG. S1. The CMA-ES algorithm can be seen as a loop of four steps: sampling of candidates from a MvN distribution, assessment of each candidate, ranking of the candidates, and updating of the MvN based on the best-ranked candidates. The sequence is repeated iteratively until a convergence threshold is achieved.

TABLE S1. Results for the 2-site Kitaev chain. The statistics of the last generation in Figs. 2(c,d) are listed for each quantity $x$, along with the corresponding median $\bar{x}$ and standard deviations $\sigma_x^{\pm}$.

| $x$ | $\bar{x}$ | $\sigma_x^+$ | $\sigma_x^-$ |
|---|---|---|---|
| $\|M_1\|$ | 0.9874 | 0.0022 | 0.0047 |
| $\|M_3\|$ | 0.9888 | 0.0013 | 0.0070 |
| $E_{\text{ex}}/\Delta$ | 0.1398 | 0.0018 | 0.0015 |
| $E_0/\Delta$ | 0.0006 | 0.0009 | 0.0004 |

TABLE S2. Statistics for the sweet spots found in the 3-site Kitaev chain, shown in Figs. 3(b–d). The top and bottom part of the table show the results for $\beta = 1$ and $\beta = 2$, respectively.

| $\beta = 1$ | | | |
|---|---|---|---|
| $x$ | $\bar{x}$ | $\sigma_x^+$ | $\sigma_x^+$ |
| $\|M\|$ | 0.9904 | 0.0024 | 0.0043 |
| $E_{\text{ex}}/\Delta$ | 0.1402 | 0.0043 | 0.0107 |
| $E_0/\Delta$ | 0.0012 | 0.0007 | 0.0007 |
| $\beta = 2$ | | | |
| $x$ | $\bar{x}$ | $\sigma_x^+$ | $\sigma_x^+$ |
| $\|M\|$ | 0.9797 | 0.0048 | 0.0050 |
| $E_{\text{ex}}/\Delta$ | 0.1667 | 0.0077 | 0.0154 |
| $E_0/\Delta$ | 0.0016 | 0.0009 | 0.0009 |

TABLE S3. Statistics for the sweet spots found in the 4- and 5-site Kitaev chains, shown in Fig. 4.

| 4-site chain | | | |
|---|---|---|---|
| $x$ | $\bar{x}$ | $\sigma_x^+$ | $\sigma_x^-$ |
| $\|M\|$ | 0.9975 | 0.0014 | 0.0024 |
| $E_{\text{ex}}/\Delta$ | 0.1212 | 0.0051 | 0.0321 |
| $E_0/\Delta$ | 0.0018 | 0.0007 | 0.0009 |
| 5-site chain | | | |
| $x$ | $\bar{x}$ | $\sigma_x^+$ | $\sigma_x^-$ |
| $\|M\|$ | 0.9986 | 0.0006 | 0.0006 |
| $E_{\text{ex}}/\Delta$ | 0.1169 | 0.0035 | 0.0028 |
| $E_0/\Delta$ | 0.0004 | 0.0004 | 0.0002 |

## C. ELECTRON-ELECTRON REPULSION AND ASYMMETRIC KITAEV CHAINS

In this Section, we include electron–electron interactions and consider asymmetric couplings between the QDs. The goal is to generalize the results shown in the main text, for symmetric Kitaev chains in the single-particle limit, and show that our tuning protocol is experimentally feasible.

We start by including an interaction term

$$H_{\text{int}} = \sum_{i=1}^{3} U_i n_{i,\uparrow} n_{i,\downarrow} \tag{S1}$$

to the Hamiltonian describing the 2-site Kitaev chain. We set $U_1 = U_3 = 5\Delta$ and assume screening in the superconducting QD to be strong enough that we can set $U_2 = 0$. We also consider asymmetries in the couplings within the chain: we keep the hopping on the left side as $t_1 = 0.5\Delta$ ($t_1^{so} = 0.2t_1$) and change the value of the coupling between the superconducting QD and the rightmost QD, $t_2 = 0.6t_1$ ($t_2^{so} = 0.6t_1^{so}$). In the many-body representation, the ground state splitting is calculated by $E_0 = |E_0^{\text{odd}} - E_0^{\text{even}}|$, where $E_0^{\text{odd,even}}$ are the odd- and even-parity ground states $|O\rangle$ and $|E\rangle$, respectively. The MP is calculated via

$$M_i = \frac{\sum_\sigma w_{i,\sigma}^2 - z_{i,\sigma}^2}{\sum_\sigma w_{i,\sigma}^2 + z_{i,\sigma}^2}, \tag{S2}$$

where $w_{i,\sigma} = \langle O| c_{i,\sigma} + c_{i,\sigma}^\dagger |E\rangle$ and $z_{i,\sigma} = \langle O| c_{i,\sigma} - c_{i,\sigma}^\dagger |E\rangle$. Finally, the excitation gap is given by $E_{\text{ex}} = E_1 - \max(E^{\text{odd}}, E^{\text{even}})$, where $E_1$ is the first excited state.

We apply the tuning method using the same loss function Eq. 4 and the same parameters as in Fig. 2, apart from $P = 50$, $W = 0.05\Delta$, and the starting values for the means of the Gaussian distributions, which are randomly drawn from the bounds $0 \leq \varepsilon_{1,3} \leq \Delta$ and $-\Delta \leq \varepsilon_2 \leq \Delta$. The statistics of the evolution of the QD levels and the MBS properties are shown in Fig. S2 as a function of the generations, showing again the evolution of the median and the standard deviations across 50 independent simulations. The quantitative values for the last generation are given in Table S4. These results corroborate those presented in the main text, showing that the tuning procedure also works when considering finite $U$ and for asymmetric Kitaev chains.

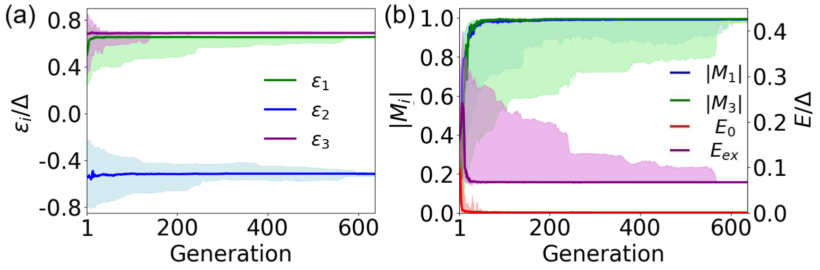


FIG. S2. Results for an asymmetric 2-site Kitaev chain with finite $U$ for 50 independent runs. The plots show the evolution of the median values (lines) and standard deviations (shades) of (a) the three QD levels and (b) $|M_1|$ (blue), $|M_3|$ (green), $E_0$ (red), and $E_{\text{ex}}$ (purple) corresponding to the best members of each generation across 50 independent simulations.

TABLE S4. Statistics for the sweet spots found in the asymmetric 2-site Kitaev chain, including finite interactions.

| $x$ | $\bar{x}$ | $\sigma_x^+$ | $\sigma_x^-$ |
|---|---|---|---|
| $\lvert M_1\rvert$ | 0.9920 | 0.0021 | 0.0146 |
| $\lvert M_3\rvert$ | 0.9944 | 0.0023 | 0.0175 |
| $E_{\text{ex}}/\Delta$ | 0.0674 | 0.0006 | 0.0006 |
| $E_0/\Delta$ | 0.0008 | 0.0007 | 0.0004 |

[1] J. Benestad, A. Tsintzis, R. S. Souto, M. Leijnse, E. van Nieuwenburg, and J. Danon, Phys. Rev. B **110**, 075402 (2024).
[2] J. Benestad, T. Rasmussen, B. Brovang, O. Krause, S. Fallahi, G. C. Gardner, M. J. Manfra, C. M. Marcus, J. Danon, F. Kuemmeth, A. Chatterjee, and E. van Nieuwenburg, Automated in situ optimization and disorder mitigation in a quantum device (2025), arXiv:2412.04997 [cond-mat.mes-hall].
[3] S. R. Katiraee-Far, Y. Matsumoto, B. Undseth, M. D. Smet, V. Gualtieri, C. V. Meinersen, I. F. de Fuentes, K. Capannelli, M. Rimbach-Russ, G. Scappucci, L. M. K. Vandersypen, and E. Greplova, Unified evolutionary optimization for high-fidelity spin qubit operations (2025), arXiv:2503.12256 [quant-ph].
[4] M. Thamm and B. Rosenow, Phys. Rev. Lett. **130**, 116202 (2023).
